# Supplementary material for: PoE-Fuse: Precision-Weighted Expert Fusion for Bi-Temporal Change Understanding
Source: arXiv:2609.37485 source file (2026-09-27)
Supplement: Supplementary file 1 [file supp_titlepage.tex]

% Supplementary title page (shared by standalone supp.tex and the optional
% combined-review build at the end of main.tex).
\begin{center}
  {\Large\bfseries PoE-Fuse: Precision-Weighted Expert Fusion\\ for Bi-Temporal Change Understanding\par}
  \vspace{4pt}
  {\Large\bfseries Supplementary Material\par}
  \vspace{22pt}
  Haruki Watase$^{\star}$, Shunya Nagashima$^{\star}$, and Takayuki Nishimura\par
  \vspace{8pt}
  Neurogica Inc., Tokyo, Japan\par
  \texttt{\{haruki.watase,shunya.nagashima,takayuki.nishimura\}@neurogica.com}\par
  \vspace{6pt}
  {\small $^{\star}$Equal contribution.\par}
\end{center}
\vspace{18pt}
